# Supplementary material for: Unveiling the multi-level structure of midgap states in Sb-doped MoX$_2$ (X = S, Se, Te) monolayers
Source: arXiv:2110.00191 ancillary file (2021-10-01)
Supplement: Supplementary file 1 [file supplemental.pdf]

# Supplemental material for: Unveiling the multi-level structure of midgap states in Sb-doped $MoX_2$ (X = S, Se, Te) monolayers

Marcos G. Menezes[1,*] and Saif Ullah[2,†]

[1] *Instituto de Física, Universidade Federal do Rio de Janeiro, Caixa Postal 68528, 21941-972 Rio de Janeiro, RJ, Brazil*

[2] *Department of Physics and Center for Functional Materials, Wake Forest University, Winston-Salem, North Carolina 27109, United States*

(Dated: September 10, 2021)

* marcosgm@if.ufrj.br

† ullahs@wfu.edu

TABLE S1. Formation energies (eV) of substitutional Sb defects and single vacancies in $MoX_2$, as calculated by the VASP code. For a definition of the formation energy and the conditions satisfied in Mo and X rich environments, see the main text. QE values are also given in the text. We present two X rich values: in the first we use the total energy per atom of the gas phase $X_2$ in the evaluation of the chemical potential $\mu_X$ (when applicable), and in the second we use the energy of the most stable bulk form of X. Notice that most of the trends are reversed when comparing these two cases. In the last column, we also report cohesive energies (eV/atom), defined as $E_c = \sum_i m_i E_i - E_{def}$, where $E_{def}$ is defined in the main text and $m_i$ and $E_i$ are the number and total energy of isolated atoms of species $i$. The cohesive energies of pure $MoX_2$ are 5.11, 4.57 and 4.01 eV for X = S, Se and Te, respectively.

| Material | Defect | Mo rich | X rich 1 | X rich 2 | Cohesive |
|---|---|---|---|---|---|
| $MoS_2$ | Sb(Mo) | 5.31 | 1.62 | 2.72 | 4.99 |
| | Sb(S) | 0.95 | 2.80 | 2.25 | 5.07 |
| | Mo vac | 7.25 | 3.56 | 4.65 | 4.99 |
| | S vac | 1.31 | 3.15 | 2.60 | 5.10 |
| $MoSe_2$ | Sb(Mo) | 4.34 | 0.73 | 2.32 | 4.46 |
| | Sb(S) | 0.94 | 2.75 | 1.95 | 4.54 |
| | Mo vac | 5.96 | 2.34 | 3.93 | 4.46 |
| | S vac | 1.56 | 3.37 | 2.57 | 4.56 |
| $MoTe_2$ | Sb(Mo) | 3.21 | - | 2.41 | 3.92 |
| | Sb(S) | 0.83 | - | 1.22 | 3.99 |
| | Mo vac | 3.70 | - | 2.91 | 3.92 |
| | S vac | 1.95 | - | 2.35 | 3.99 |

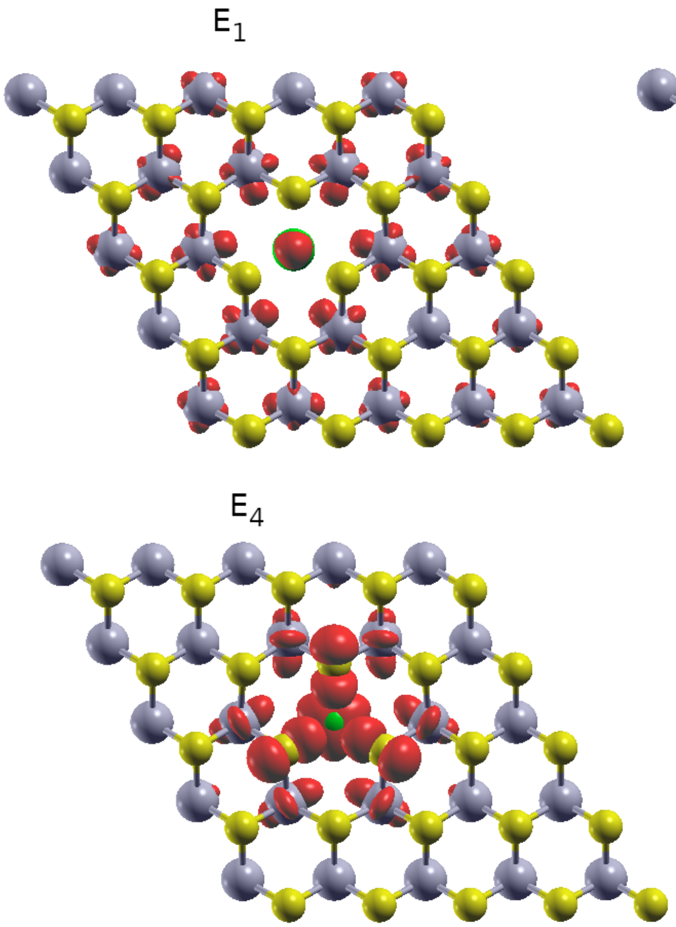


FIG. S1. Local density of states (LDOS) isosurfaces for the impurity levels induced by the Sb(Mo) substitution in $MoSe_2$. The levels are arranged in increasing energy, as described in the main text. The isosurfaces, shown in red, correspond to 10% of the maximum value found in each case. The Sb impurity is represented as a green sphere, while the Mo and Se atoms are represented by gray and yellow spheres, respectively.

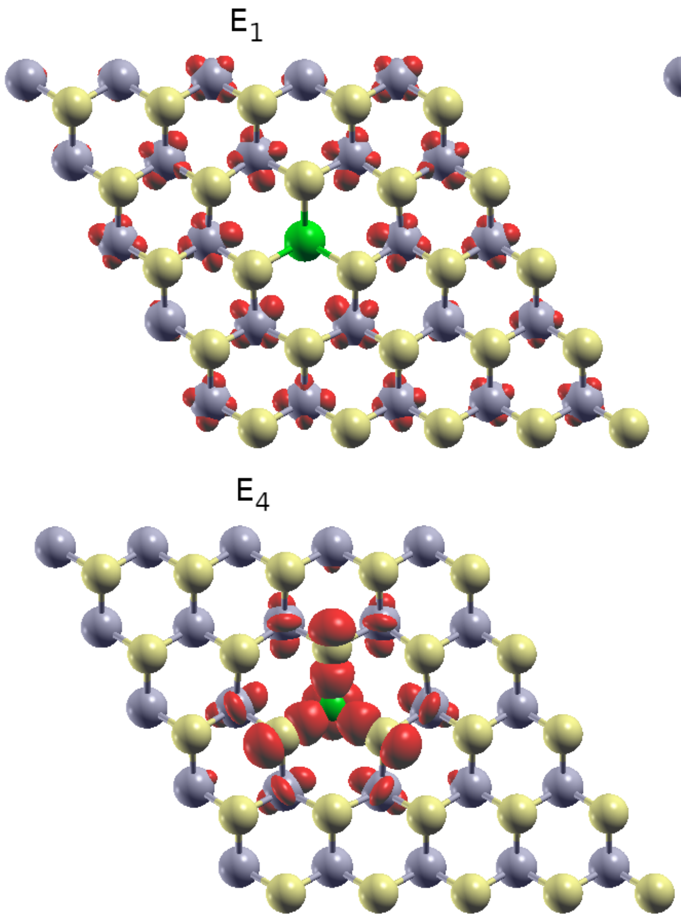


FIG. S2. Local density of states (LDOS) isosurfaces for the impurity levels induced by the Sb(Mo) substitution in $MoTe_2$. The isosurface parameters and color codes are the same as in Fig. **??**. Note that, for this case, the contribution from the 5$s$ orbital of Sb to the $E_1$ level is not visible for this particular isosurface, but it can be identified in the PDOS calculations shown in Fig. 3 of the main text.

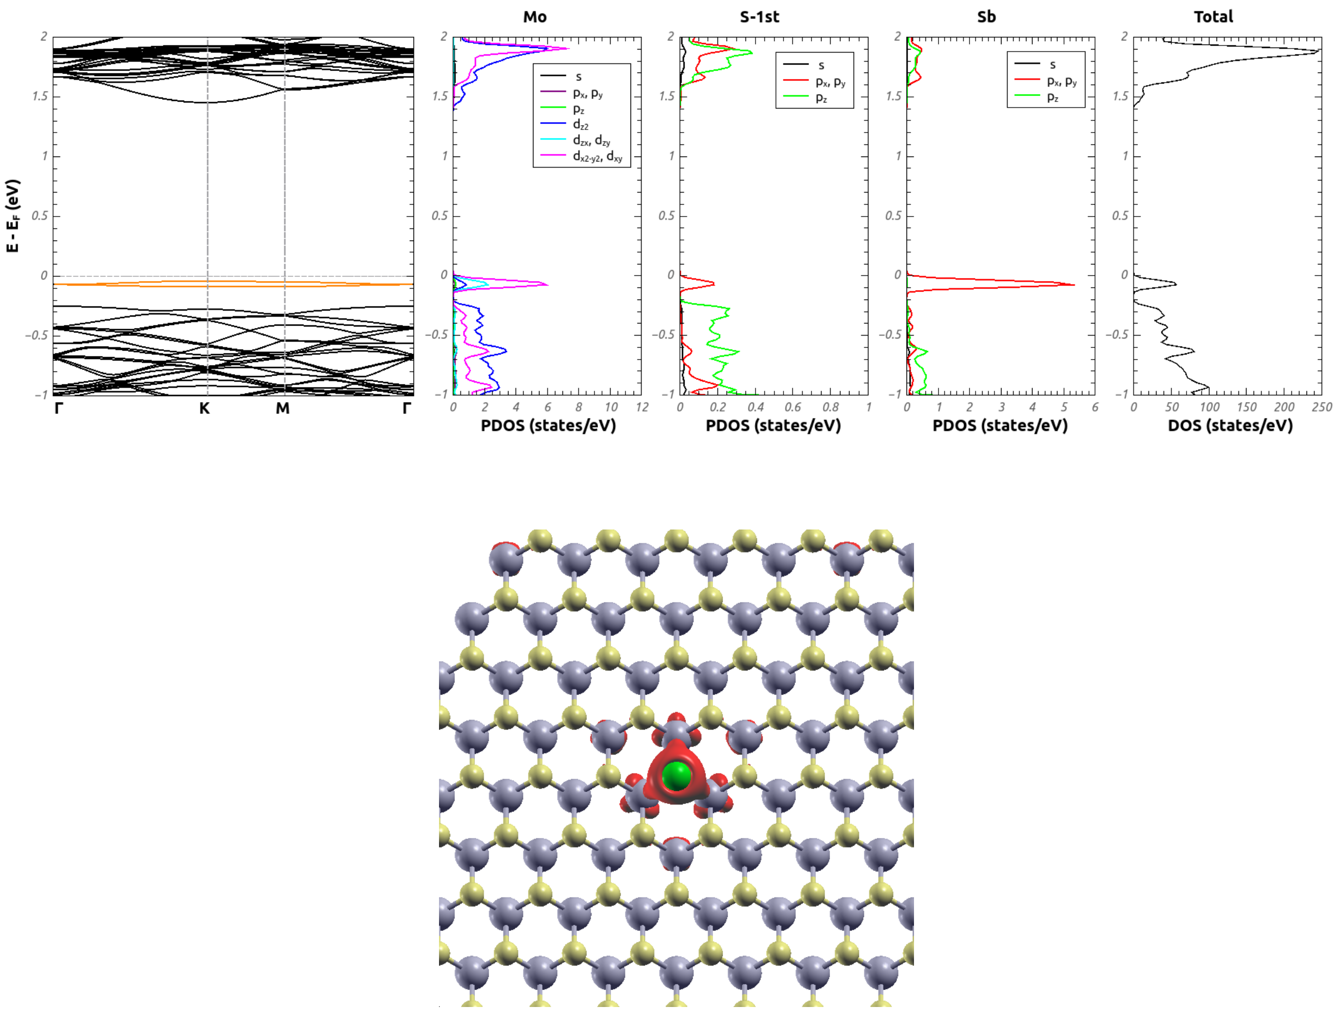


FIG. S3. Electronic properties of a Sb(S) substitutional impurity in $MoS_2$. *Top*: Band structure and projected density of states (PDOS). Two near-degenerate levels are found inside the gap and are highlighted in orange. The binding energy, as measured from the top of the valence band, is 0.16 eV. The projections show contributions from orbitals of the impurity itself (Sb), its neighboring S atom in the opposing layer (S-1st) and the sum over neighboring Mo atoms (Mo). The total DOS is also displayed. Interestingly, in this case the $5p_x$ and $5p_y$ orbitals of Sb participate in the composition of the impurity states, in contrast to the Sb(Mo) defect, where only the $5s$-orbital is involved. The band gap is 1.68 eV, which is slightly higher than the value found in the pristine system (see Table I in the main text). *Bottom* Local density of states (LDOS) isosurface for the pair of impurity levels. The isosurface parameters and color codes are the same as in Fig. **??**. These properties suggest that Sb(S) behaves as a standard acceptor impurity with a degenerate ground state.

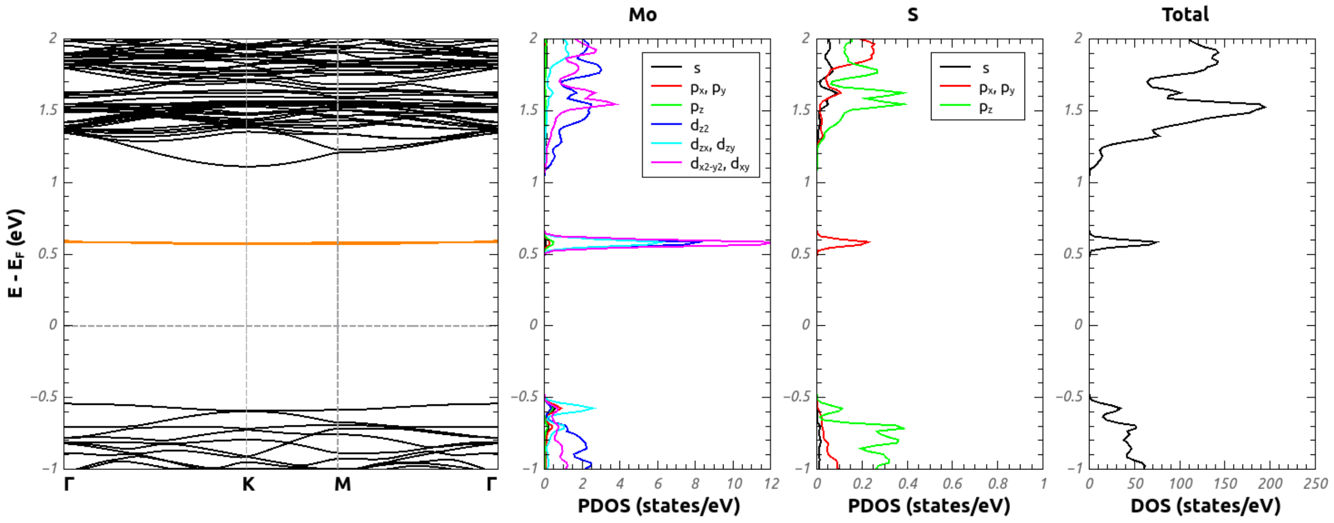


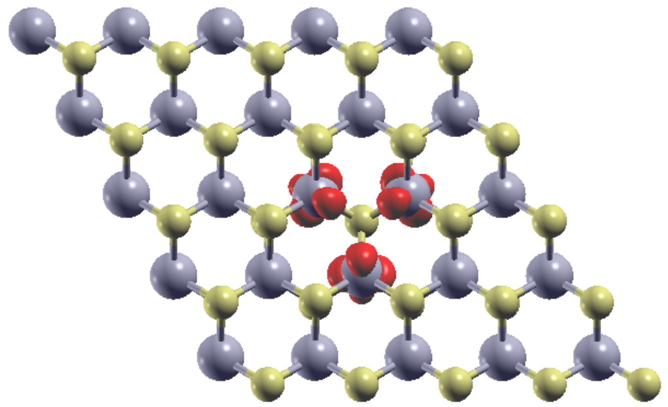

FIG. S4. Electronic properties of a single S vacancy in $MoS_2$. *Top*: Band structure and projected density of states (PDOS). As in the Sb(S) defect, two near-degenerate levels are found inside the gap and are highlighted in orange. However, these levels are much deeper, with an energy of 1.12 eV measured from the valence band edge. The projections show contributions from orbitals of the neighboring S atom in the opposing layer (S) and the sum over neighboring Mo atoms (Mo). The band gap is 1.66 eV, which is identical to that of the pristine case (see Table I in the main-text). The total DOS is also displayed. *Bottom* Local density of states (LDOS) isosurface for the pair of impurity levels. The isosurface parameters and color codes are the same as in Fig. **??** and the vacancy is located at the center of the triangular-shaped profile. This profile is very similar to that found for the Mo atoms in the Sb(S) defect, suggesting that the defect states in the latter case result from a rehybridization of vacancy defect states and $5p$ orbitals from Sb.

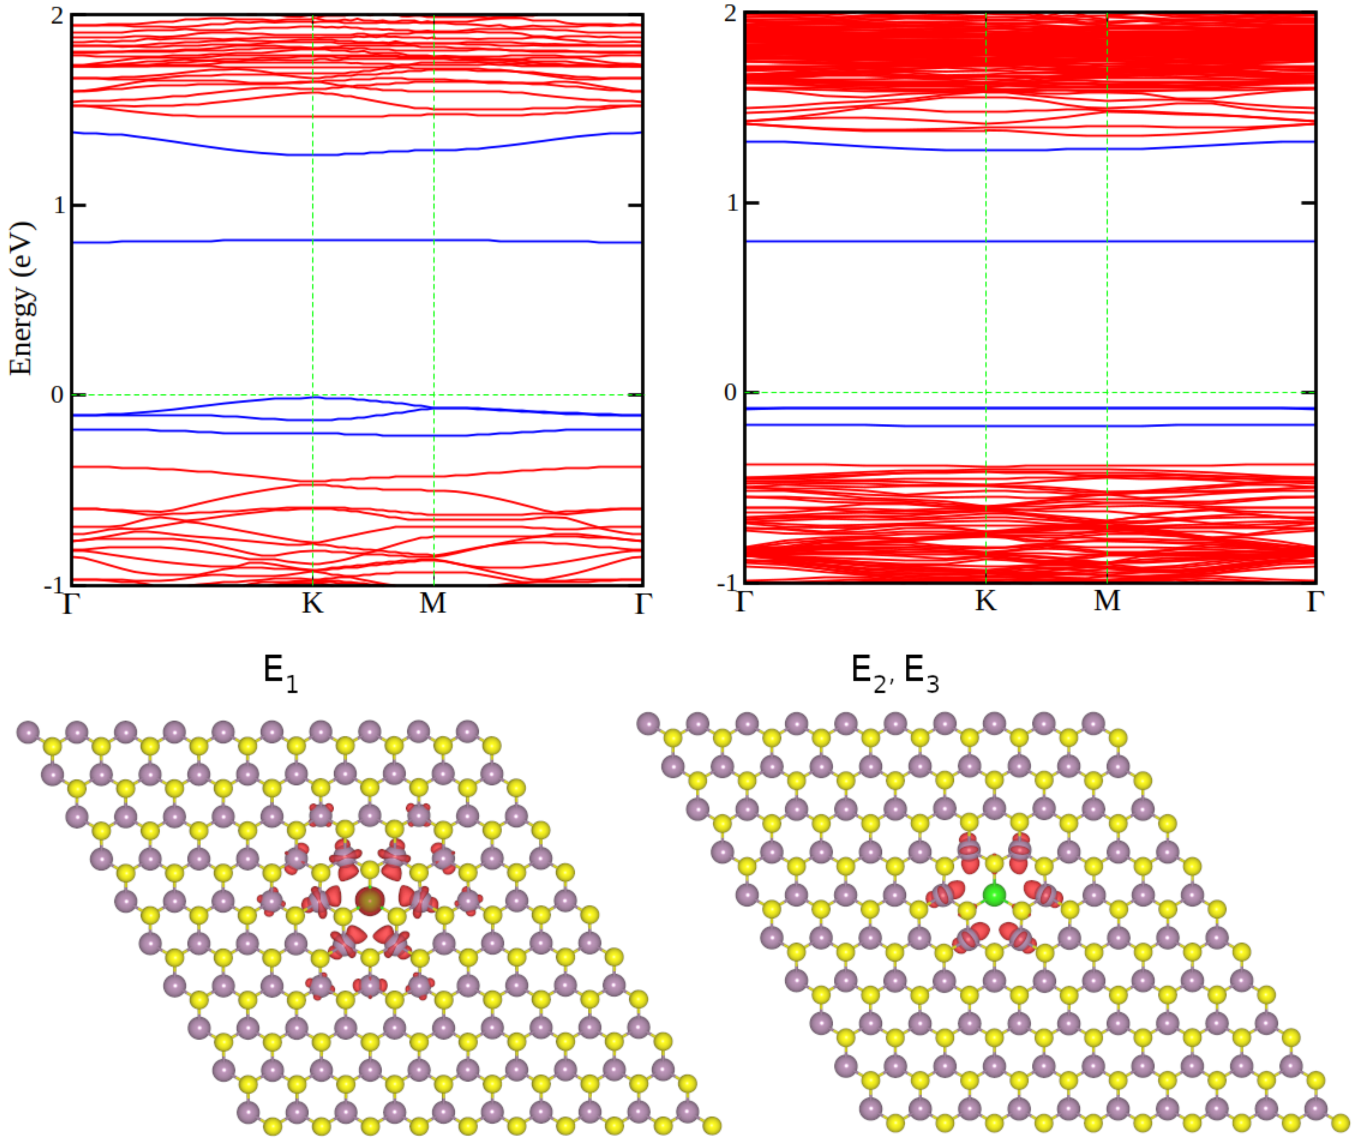


FIG. S5. *Top:* Band structures of Sb(Mo) doped $MoS_2$ in a $5\times5$ (left) and $10\times10$ supercell (right). These supercells correspond to atomic defect concentrations of 4% and 1%, respectively, with respect to the total number of Mo atoms. Both calculations were performed with the VASP code and the effects of the spin-orbit interaction are neglected. *Bottom:* Local density of states isosurfaces for the $E_1$ and $E_2, E_3$ levels in the $10\times10$ cell. The isosurface parameters and color codes are the same as in Fig. **??**. Note that the structure of the impurity levels is preserved and the weak dispersion of levels $E_1$, $E_2$ and $E_3$ disappears in the larger cell, indicating that the residual interaction between the impurity and its periodic images is practically eliminated.

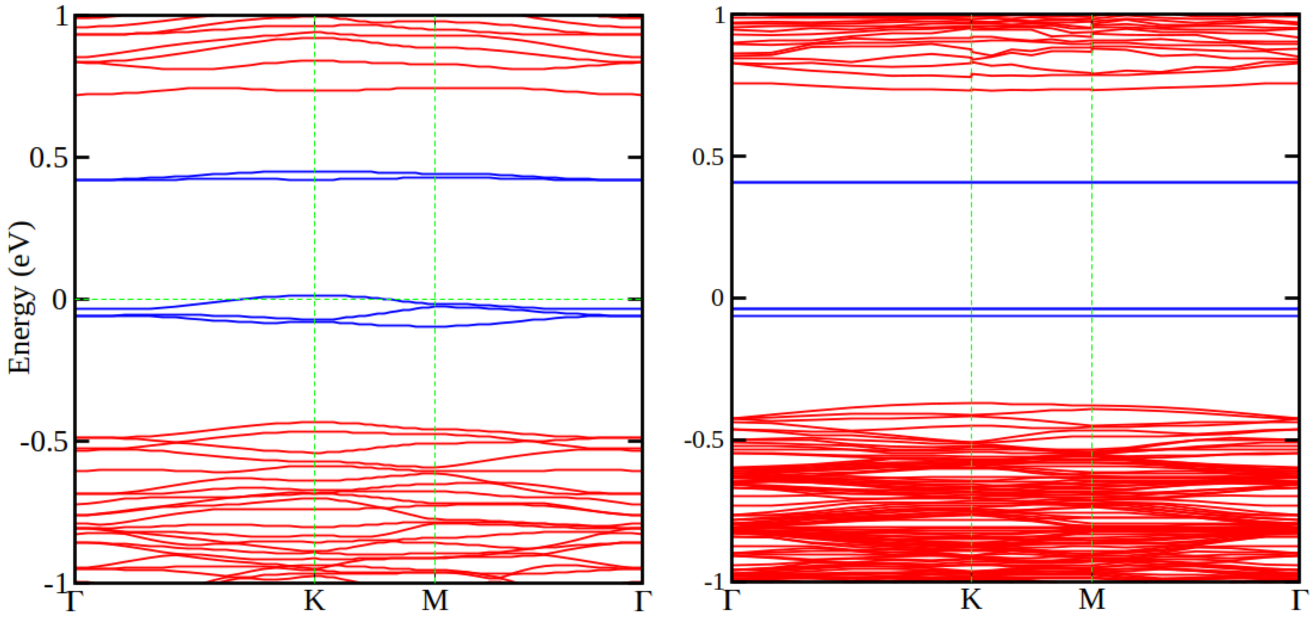


FIG. S6. Band structures for a Mo vacancy in $MoTe_2$ in a $5 \times 5$ (left) and $10 \times 10$ supercell (right). These supercells correspond to atomic defect concentrations of 4% and 1%, respectively, with respect to the total number of Mo atoms. Both calculations were performed with the VASP code and the effects of the spin-orbit interaction are neglected. Notice that, as in Fig. **??**, the dispersion of the impurity levels is eliminated in the larger supercell, but their structure is preserved.

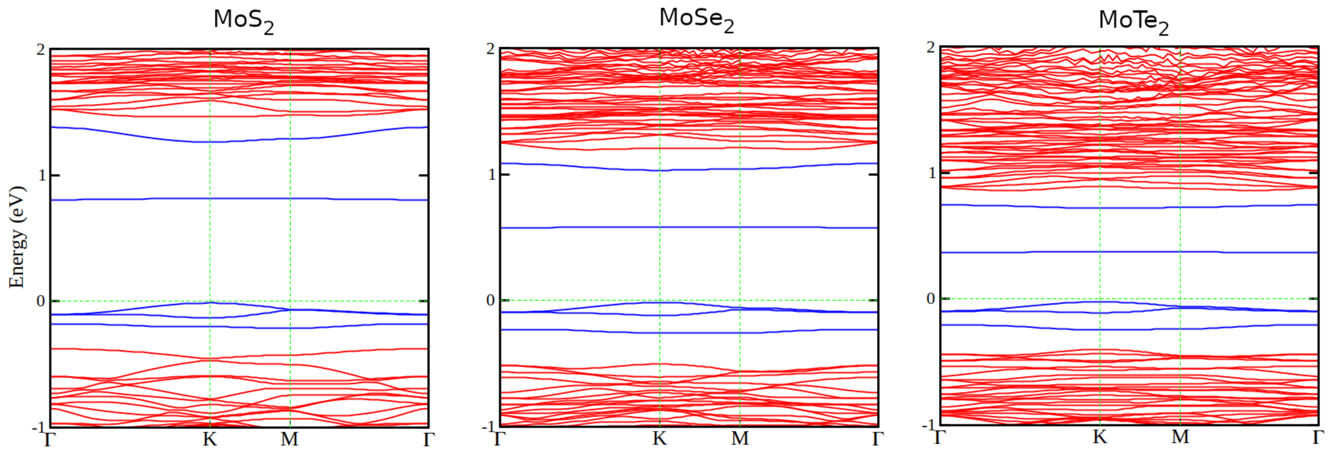


FIG. S7. Band structures of Sb(Mo) doped $MoX_2$ calculated with the VASP code in a $5 \times 5$ supercell. The electronic structure of the impurity levels (highlighted in blue) agrees with our calculations from QE, displayed in the main text.

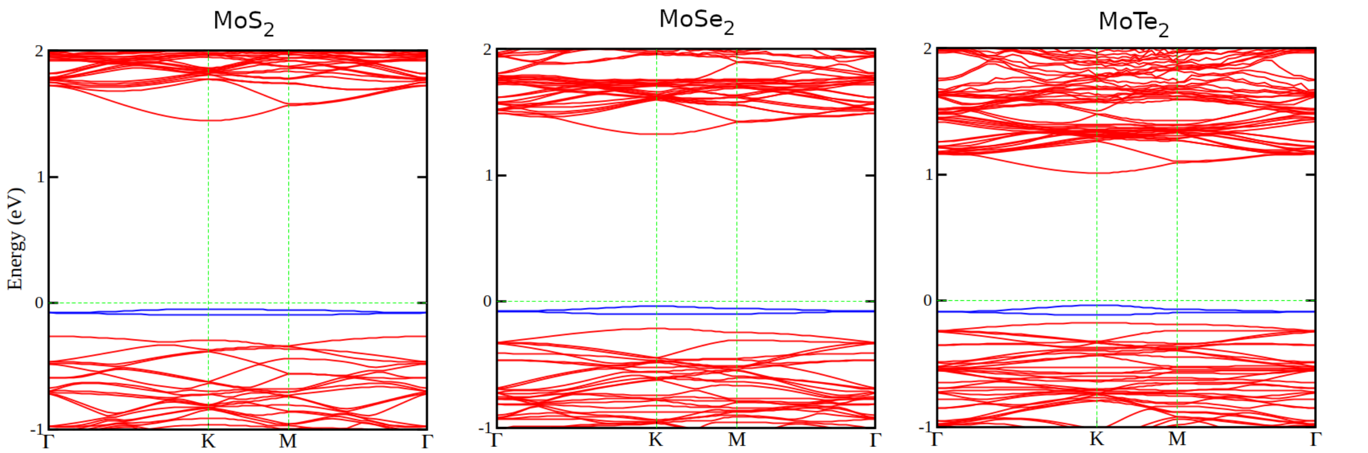


FIG. S8. Band structures of Sb(X) doped $MoX_2$ calculated with the VASP code in a $5 \times 5$ supercell. The electronic structure of the impurity levels (highlighted in blue) agrees with our calculation for $MoS_2$ done in QE, shown in Fig. S3.

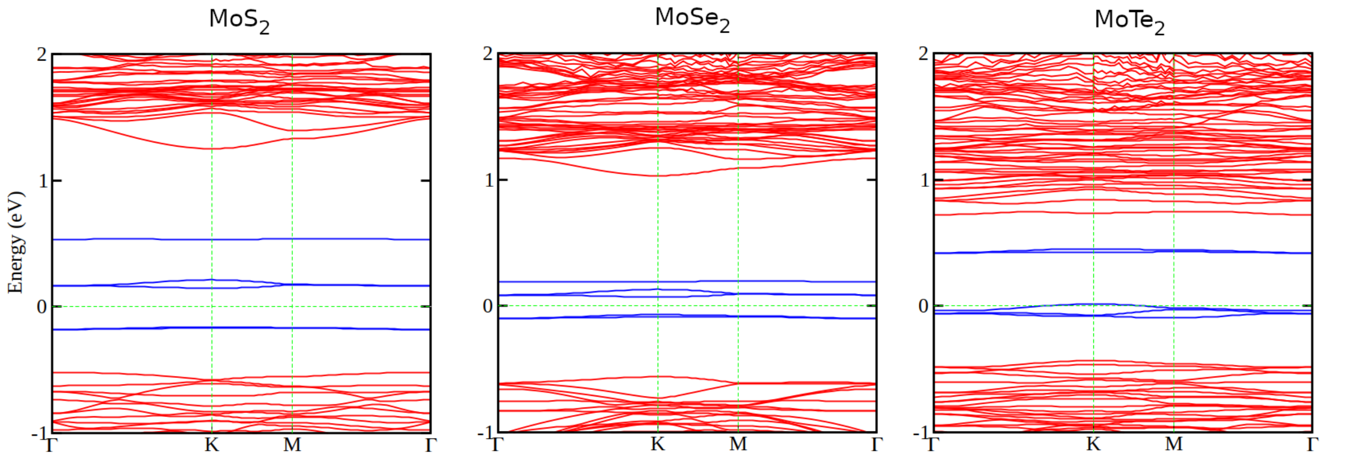


FIG. S9. Band structures of $MoX_2$ with a single Mo vacancy calculated with the VASP code in a $5 \times 5$ supercell. The electronic structure of the impurity levels (highlighted in blue) agrees with our calculations from QE for $MoS_2$, displayed in the main text.

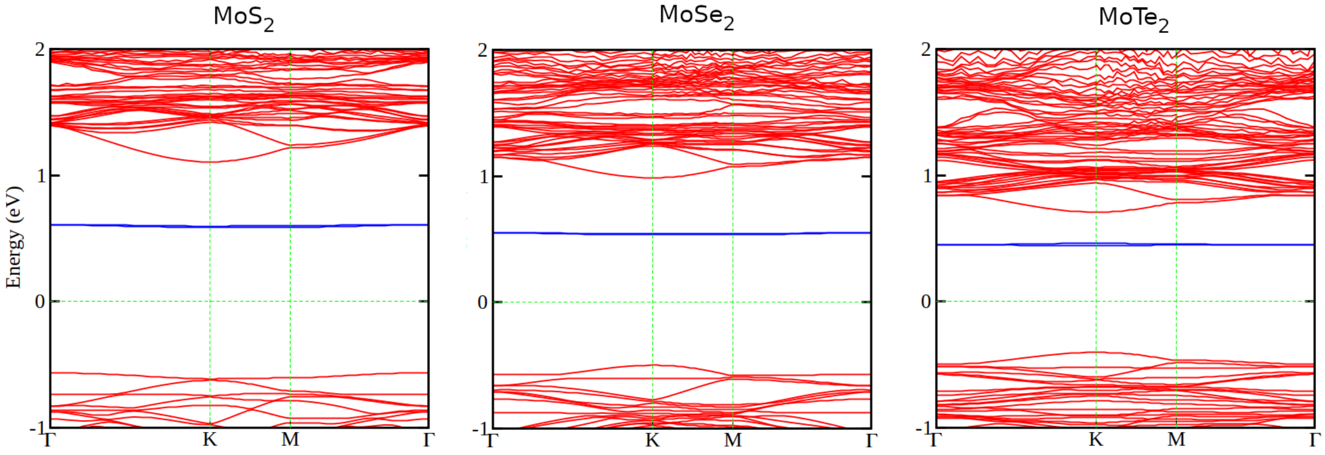


FIG. S10. Band structures of $MoX_2$ with a single X vacancy calculated with the VASP code in a $5 \times 5$ supercell. The electronic structure of the impurity levels (highlighted in blue) agrees with our calculations from QE for $MoS_2$, shown in Fig. S4.

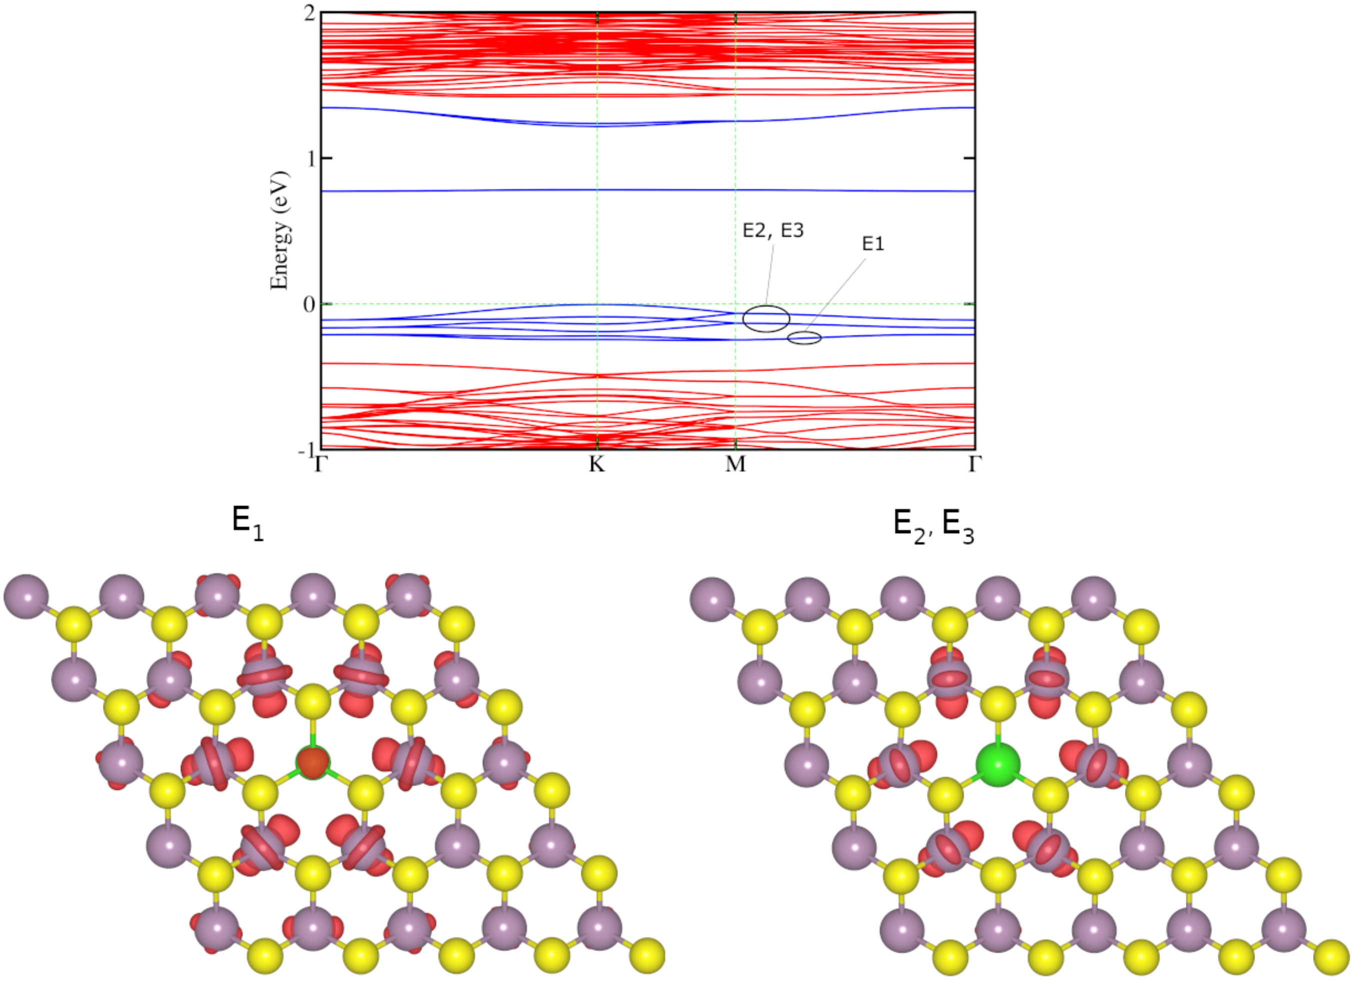


FIG. S11. *Top:* Band structure of Sb(Mo) doped $MoS_2$ with spin-orbit coupling in a $5 \times 5$ supercell (same as the bottom right panel in Fig. 8 of the main text). *Bottom:* Local density of states isosurfaces for the $E_1$ and $E_2, E_3$ levels. The isosurface parameters and color codes are the same as in Fig. **??** and the LDOS is integrated over the entire energy range of each splitting. The calculations were performed with the VASP code. Notice that the structure of the impurity-level wavefunctions is preserved in the presence of SOC.
